# Supplementary material for: A Model-Driven-Engineering Approach for Detecting Privilege Escalation in IoT Systems
Source: arXiv:2205.11406 source file (2022-05-23)
Supplement: Supplementary file 1 [file Appendix1.tex]

\let\svaddcontentsline\addcontentsline
\renewcommand\addcontentsline[3]{%
  \ifthenelse{\equal{#1}{lof}}{}%
  {\ifthenelse{\equal{#1}{lot}}{}{\svaddcontentsline{#1}{#2}{#3}}}}
  
\begin{appendix}

%\chapter{Prolog Rules for Case 1}\label{appendix1}
  \section{Prolog Rules - Case 1 of Over-Privilege}\label{appendix1}
  \addcontentsline{loaf}{section}{\protect\numberline{A} Prolog Rules for Case 1}
    \lstinputlisting[style=Prolog-pygsty, caption=Prolog Rules for Case 1]{"./Code/PrologCase1.pl"}
\end{appendix}
